# Supplementary material for: NARU: A Benchmark for NARrative Evolution and Cultural Nuance Understanding in Japanese Extreme Long Video
Source: arXiv:2608.13210 source file (2026-08-13)
Supplement: Supplementary file 1 [file appendix.tex]

    \appendices
    
    \section{Filtering Algorithm}
    \label{app:filtering}
    
    The incremental diversity filtering procedure is summarized in Algo.~\ref{alg:diversity_filter}. We use the text-embedding-3 model to encode video titles and descriptions into fixed-length vectors. A candidate video is added only if its cosine similarity to all previously selected samples is below a fixed threshold $\tau$ of 0.85. The initial seed set size is set to 30.
    
    \begin{algorithm}[h]
    \caption{Incremental Semantic Diversity Filtering}
    \label{alg:diversity_filter}
    \begin{algorithmic}[1]
    \Require Stream of candidates $\mathcal{D}_{in}$, Embedding model $\phi(\cdot)$, Cosine Similarity Threshold $\tau$, Initial Set Size Threshold $q$
    \Ensure Filtered dataset $\mathcal{S}$
    \State $\mathcal{S} \leftarrow \text{LoadCachedState}()$ \Comment{Initialize with persisted data}
    \For{$x \in \mathcal{D}_{in}$}
        \State $\mathbf{v}_x \leftarrow \phi(x)$ \Comment{Generate normalized embedding}
        \If{$|\mathcal{S}| < q$}
            \State $\mathcal{S} \leftarrow \mathcal{S} \cup \{(x, \mathbf{v}_x)\}$
        \Else
            \State Let $\mathcal{V}_{\mathcal{S}}$ be the set of vectors currently in $\mathcal{S}$
            \State $\sigma_{\max} \leftarrow \max_{\mathbf{v}_s \in \mathcal{V}_{\mathcal{S}}} (\mathbf{v}_x^\top \mathbf{v}_s)$ \Comment{Compute max cosine similarity}
            \If{$\sigma_{\max} \leq \tau$}
                \State $\mathcal{S} \leftarrow \mathcal{S} \cup \{(x, \mathbf{v}_x)\}$ \Comment{Add distinctive sample}
                \State $\text{UpdateCache}(\mathcal{S})$
            \Else
                \State \textbf{continue} \Comment{Reject redundant sample}
            \EndIf
        \EndIf
    \EndFor
    \State \Return $\mathcal{S}$
    \end{algorithmic}
    \end{algorithm}
    
    \section{Task-oriented Annotation}
    \label{app:task_annotation}
    
    The following sections detail the specific schemas and prompts used by \textbf{Narrative Thread Agent} and  \textbf{Cultural Agent}. 
    
    \subsection{Narrative Thread Agent Details}
    \label{app:task_annotation:narrative_agent}
    
    The Narrative Thread Agent is responsible for constructing the narrative layer by identifying character roles and causal threads.
    
    \subsubsection{Character Role Schema}
    The agent classifies characters based on their functional role in the story structure:
    \begin{itemize}
        \item \textbf{Focal Character (FOCAL):} Central figures who possess personal agency, experience internal states, and undergo observable changes (arcs) throughout the narrative. They carry the main conflict.
        \item \textbf{Anchor Character (ANCHOR):} Characters who facilitate the narrative flow, provide information, or guide interactions but remain static in their stance and internal state (e.g., narrators, hosts, interviewers).
        \item \textbf{Background Character (BACKGROUND):} Characters present only to reinforce context or visual setting, without direct intervention in the narrative thread.
    \end{itemize}
    
    \subsubsection{Narrative Thread and Event Schema}
    A narrative thread is defined as a minimal story unit consisting of causally connected events. The agent categorizes key turning points into three domains:
    
    \begin{enumerate}
        \item \textbf{Relational Events (Connection Changes):}
        \begin{itemize}
            \item \textit{Alliance:} Entities joining forces, agreeing, or merging.
            \item \textit{Conflict:} Collision of interests, onset of disputes, or escalation.
            \item \textit{Reversal:} A decisive event where power dynamics flip or flow changes direction.
        \end{itemize}
        
        \item \textbf{Epistemic Events (Cognitive Changes):}
        \begin{itemize}
            \item \textit{Deception:} False information or traps establishing incorrect perceptions as fact.
            \item \textit{Insight:} Fragmented information connecting to solve a mystery or lead to realization.
        \end{itemize}
        
        \item \textbf{Systemic Events (Environmental Changes):}
        \begin{itemize}
            \item \textit{Conclusion:} A state becoming finalized (e.g., verdict, deal closed).
            \item \textit{Intervention:} External or higher powers forcing a change in the natural flow.
            \item \textit{Origin:} The initial appearance of a problem, trend, disaster, etc.
        \end{itemize}
    \end{enumerate}
    
    \subsubsection{System Prompt (Narrative)}
    The following system prompt is used to instruct the Narrative Thread Agent:
    
    \begin{lstlisting}
    提供された動画を詳細に分析し、指定されたスキーマに従って**ナラティブ(narrative)キャプション**を抽出してください。既存のMLLM注釈（参考情報）と文字起こし(利用可能な場合)を補助として活用してください。
    
    **分析指示:**
    - 「キャラクターの役(character\_roles)」キャラクターを、内面的変容と葛藤を担う主体、一貫した立場から情報伝達や誘導を行う進行役、および場面の文脈補完のみに留まる背景の三種類に抽出すること
    - 「叙述展開(narrative\_threads)」の抽出と構成
      a. 相互に関連する離散的なイベントの連なりによって形成される、意味的に完結した最小の叙事単位として特定すること
      b. 動画の全体的な流れからこの部分だけを取り出したとしても、背景知識なしに「誰が、いつ、何をして、どうなったか」という一貫したストーリーや意図が成立する独立性を維持すること
      c. 各展開内で、一連のイベントが織りなす文脈、因果関係、および結果を包括的な要約として記述すること
    
    **参考情報の扱い:**
    - チャンク境界付近のイベントは記述が途切れている(TRUNCATEDと表記)可能性があるため、その不完全性を考慮すること
    - イベントや出来事の文脈を深く理解するために、記述に含まれる対象の詳細情報について、以下の定義リストを補助として活用すること
    {Entity Definition Reference}
    - 各区間の役割において、以下の定義を補助情報として参照すること
    {Segment Type Reference}
    
    **出力要件:**
    - 指定されたスキーマ構造に従って応答すること
    - すべて日本語で応答すること
    \end{lstlisting}
    
    \newpage
    
    \subsection{Cultural Agent Details}
    \label{app:cultural_agent}
    
    The Cultural Schema Agent focuses on interpreting high-context implicit signals.
    
    \subsubsection{Cultural Dimensions Schema}
    The agent annotates the content across five specific cultural dimensions:
    
    \begin{enumerate}
        \item \textbf{Aizuchi (Interjections):}
        Captures the usage of short interjections (e.g., "Hai", "Un", "Hee") not merely as affirmation but as functional signals for:
        \begin{itemize}
            \item \textit{Active Listening (Keichou)}
            \item \textit{Agreement (Doui)}
            \item \textit{Emotional Reaction (Kanjou hannou)}
            \item \textit{Conversation pacing/facilitation}
        \end{itemize}
    
        \item \textbf{Kuuki wo Yomu (Reading the Air):}
        Identifies "Social Context" events where participants respond to implicit rules or atmosphere:
        \begin{itemize}
            \item \textit{Situation:} The observed social situation.
            \item \textit{Unspoken Meaning:} Implicit social rules or shared sentiments.
            \item \textit{Cultural Significance:} The significance of the atmosphere and social dynamics.
        \end{itemize}
    
        \item \textbf{Tatemae vs. Honne (Subtext Interpretation):}
        Analyzes the divergence between surface speech and underlying intent:
        \begin{itemize}
            \item \textit{Literal Text (Tatemae):} The spoken words.
            \item \textit{Implied Meaning (Honne):} The true intent or subtext inferred from context (e.g., social consideration, self-defense, humility).
            \item \textit{Cultural Context:} Interpretation based on cultural norms.
        \end{itemize}
    
        \item \textbf{Cultural References:}
        Identifies specific references to Japanese culture:
        \begin{itemize}
            \item \textit{Reference:} The object, action, or concept (e.g., dialects, customs, historical figures).
            \item \textit{Explanation:} Detailed explanation of the reference.
            \item \textit{Significance:} Its role in the current context.
        \end{itemize}
    
        \item \textbf{Sentiment and Dynamics:}
        Captures the "flow" of the interpersonal atmosphere:
        \begin{itemize}
            \item \textit{Emotional Tone:} The mood governing the segment (e.g., tension, harmony, awkwardness).
            \item \textit{Cultural Appropriateness:} Whether behavior is appropriate for the TPO (Time, Place, Occasion).
            \item \textit{Interpersonal Dynamics:} Status of relationships (power gradients, distance/intimacy).
        \end{itemize}
    \end{enumerate}
    
    \subsubsection{System Prompt (Cultural)}
    The following system prompt is used to instruct the Cultural Schema Agent:
    
    \begin{lstlisting}
    提供された動画を詳細に分析し、指定されたスキーマに従って文化的理解データを抽出してください。既存のMLLM注釈と文字起こし(利用可能な場合)を参考コンテキストとして活用してください。
    
    **分析指示:**
    1. 動画全体を注意深く視聴し、会話と社会的文脈に特に注意を払う
    2. 相槌の使用パターンを識別:「はい」「うん」「ええ」「そうですね」などの機能的役割を分析
    3. 空気を読む場面を検出:明示されていない社会的ルールや共有された感情、場の雰囲気を特定
    4. 建前と本音を解釈:文字通りの発話と暗示された真意の違いを分析
    5. 文化的参照を識別:文化的対象、行動、言及とその意義を説明
    6. 感情トーンと対人関係性の推移を評価
      単なる全体の要約ではなく、区間内での雰囲気の変化を捉えること
      a. 安定的: 雰囲気が終始一貫している場合は、リストに単一の評価を含める
      b. 変化あり: 途中で雰囲気が劇的に変化する場合（例：和やかな雑談から緊張した対立へ）は、その推移を表現するために複数の評価を時系列順にリスト化する
      c. 該当なし: イントロ、広告、風景描写のみなど、分析に値する対人関係や感情的文脈が存在しない場合は、無理に出力せず空リストとする
    
    **参考情報の扱い:**
    - チャンク境界付近のイベントは記述が途切れている(TRUNCATEDと表記)可能性があるため、その不完全性を考慮すること
    - イベントや出来事の文脈を深く理解するために、記述に含まれる対象の詳細情報について、以下の定義リストを補助として活用すること
    {Entity Definition Reference}
    - 各区間の役割において、以下の定義を補助情報として参照すること
    {Segment Type Reference}
    
    **出力要件:**
    - 指定されたschema構造に従って応答すること
    - タイムスタンプは秒単位で記録すること
    - 文化的文脈における適切性と意義を明確に説明すること
    - すべて日本語で応答すること
    \end{lstlisting}
    
    \section{Iterative Debiasing: The Solver--Critic Loop}
    \label{app:solver_critic}
    
    The iterative debiasing stage (Sec.~\ref{sec:method:refinement}) is realized as a Solver--Critic loop over the generated multiple-choice questions.
    It couples three agents: a Blind Solver Agent that attempts each question with the video withheld, a Diagnostic Agent that attributes any success to a specific vulnerability, and a Distractor Patching Agent that rewrites the implicated distractors.
    An item is vulnerable exactly when the Blind Solver Agent still selects the correct answer without the video, so the loop neutralizes vulnerabilities rather than raising difficulty in the abstract.
    The correct answer and the question stem are held immutable throughout, and only distractors are edited, which preserves ground-truth validity.\jianlang{TBD: edit runs on all three include stem and correct-answer; -> change the claim and cite the second human verification stage (\ref{sec:method:quality}) as the actual drift guard ??}
    The Blind Solver Agent is realized as an ensemble of $N$ samples from one base model, decoded at temperatures on a fixed schedule that rises convexly with the sample index while top-$p$ tapers, so the ensemble probes conservative and exploratory shortcuts at once.
    
    \begin{algorithm}[h]
    \caption{Iterative Debiasing via the Solver--Critic Loop}
    \label{alg:solver_critic}
    \begin{algorithmic}[1]
    \Require MCQ batch $\mathcal{Q}$, Blind-Solver ensemble size $N$, maximum rounds $R$
    \Ensure Debiased batch $\mathcal{Q}$ \Comment{stem and correct answer immutable; only distractors change}
    \State $\mathcal{O} \leftarrow \mathcal{Q}$ \Comment{items still open for refinement}
    \For{$r = 1$ \textbf{to} $R$}
        \For{$q \in \mathcal{O}$} \Comment{Blind Solver Agent: video withheld, $V = \emptyset$}
            \State $C_q \leftarrow \{\, i : \text{BlindSolver}_i(q) \text{ selects the correct answer} \,\}$ \Comment{$N$ diversified samples}
        \EndFor
        \State $\mathcal{H} \leftarrow \{\, q \in \mathcal{O} : C_q = \emptyset \,\}$ \Comment{no sample succeeds $\Rightarrow$ not vulnerable}
        \State $\mathcal{O} \leftarrow \mathcal{O} \setminus \mathcal{H}$ \Comment{freeze non-vulnerable items}
        \If{$\mathcal{O} = \emptyset$}
            \State \textbf{break} \Comment{blind accuracy approaches chance}
        \EndIf
        \State $\mathcal{P} \leftarrow \text{Diagnose}\big(\{\, (q,\ \{\text{reasoning}(i) : i \in C_q\}) : q \in \mathcal{O} \,\}\big)$ \Comment{Diagnostic Agent: reads only successful solvers; one Refine Plan per item, naming its vulnerability}
        \For{$p \in \mathcal{P}$}
            \State $e \leftarrow \text{Patch}(p)$ \Comment{Distractor Patching Agent: one plan $\Rightarrow$ one distractor}
            \State $\text{Apply}(e, q_p)$ \Comment{overwrite the named distractor only}
        \EndFor
    \EndFor
    \State \Return $\mathcal{Q}$
    \end{algorithmic}
    \end{algorithm}
    
    Each patch names the Refine Plan it addresses and the distractor it targets, so every committed change is traceable to a single diagnosed vulnerability.
    Patches that reference an unknown plan or fall outside the plan's target are rejected and regenerated.
